# Supplementary material for: Nonlinear Predictive Control on a Heterogeneous Computing Platform
Source: arXiv:1710.08737 source file (2017-10-24)
Supplement: Supplementary file 1 [file appendix_crane_model.tex]

\section{Gantry crane model and OCP parameters} \label{sec:crane_ode}

%Gantry crane ODE model:

\begin{subequations}
\begin{gather*}
\begin{aligned}
\dot{x}(1) = & \ x(2), \enspace \dot{x}(3) =  x(4), \enspace  \dot{x}(5) =  x(6), \enspace \dot{x}(7) =  x(8)\\
\dot{x}(2) = & -(0.22\, \sin (x(5))\, {x(6)}^2 + 15.85\, u(1) -44.17\, x(2) \\ &  + 4.61 {\cos (x(5))}\, \sin (x(5)))/(0.47 {\cos (x(5))}^2 - 3.84) \\ 
%\dot{x}(3) = & x(4) \\
\dot{x}(4) = &- (0.22\, \sin (x(7))\, {x(8)}^2 + 15.85\, u(2) - 43.02\, x(4) \\ &  + 4.61 {\cos (x(7) )} \sin (x(7) ))/ (0.47 {\cos(x(7))}^2 - 2.13)\\
%\dot{x}(5) = & x(6), \quad \dot{x}(7) =  x(8) \\
\dot{x}(6) = & (0.22\, \cos (x(5))\, \sin (x(5))\, {x(6)}^2 + \\ & + 37.67  \sin (x(5))  + 15.85 u(1) \cos (x(5)) -\\ & - 44.17\, x(2) \cos (x(5)))/(0.22\, {\cos(x(5))}^2 - 1.80)  \\
%\dot{x}(7) = & x(8) \\ 
\dot{x}(8) = & (0.22\, \cos (x(7))\, \sin (x(7))\, {x(8)}^2+ \\ & + 20.89 \sin (x(7)) +  15.85 u(2) \cos (x(7)) -\\ & - 43.02\, x(4) \cos (x(7)))/(0.22\, {\cos (x(7))}^2 - 1.00) \\
\end{aligned}
\end{gather*}
\end{subequations}

%\begin{subequations}
%\begin{gather*}
%\begin{aligned}
%\dot{x}(1) = & \ x(2), \enspace \dot{x}(3) =  x(4), \enspace  \dot{x}(5) =  x(6), \enspace \dot{x}(7) =  x(8)\\
%\dot{x}(2) = & -(0.2209\, \sin (x(5))\, {x(6)}^2 + 15.8538\, u(1) - \\ & -44.1705\, x(2) + 4.6107\, \cos (x(5))\, \sin (x(5)))/ \\ & /(0.47 {\cos (x(5))}^2 - 3.84) \\
%%\dot{x}(3) = & x(4) \\
%\dot{x}(4) = &- (0.2209\, \sin (x(7))\, {x(8)}^2 + 15.8538\, u(2) - \\ &- 43.0223\, x(4) + 4.6107\, \cos (x(7) ) \sin (x(7) ))/ \\ & /(0.47 {\cos(x(7))}^2 - 2.13)\\
%%\dot{x}(5) = & x(6), \quad \dot{x}(7) =  x(8) \\
%\dot{x}(6) = & (0.2209\, \cos (x(5))\, \sin (x(5))\, {x(6)}^2 + \\ & + 37.67  \sin (x(5))  + 15.8538 u(1) \cos (x(5)) -\\ & - 44.1705\, x(2) \cos (x(5)))/ \\ & /(0.2209\, {\cos(x(5))}^2 - 1.8048) \\
%%\dot{x}(7) = & x(8) \\ 
%\dot{x}(8) = & (0.2209\, \cos (x(7))\, \sin (x(7))\, {x(8)}^2+ \\ & + 20.8953 \sin (x(7)) +  15.8538 u(2) \cos (x(7)) -\\ & - 43.02\, x(4) \cos (x(7)))/ \\ & /(0.2209\, {\cos (x(7))}^2 - 1.0011) \\
%\end{aligned}
%\end{gather*}
%\end{subequations}

%OCP parameters:

$$\hat{x} = [0, 0, 0, 0, \pi /3, 0, \pi /4, 0]^T, S_d = 0_{n,m}$$
$$Q_d = \operatorname{diag}(10,0,10,0,10,0,10,0), P_d=Q_d$$
$$R_d = \operatorname{diag}(0.01, 0.01), J =  0_{v,n}, \textrm{where } v=4$$
$$E =  \begin{bmatrix}
1 & 0 & -1 & 0 \\
0 & 1 & 0 & -1
\end{bmatrix}^T, d = \begin{bmatrix} 2 & 2 & 2 & 2 \end{bmatrix}^T$$
%\begin{equation}
%M=
%\left(\begin{array}{c} \mathrm{x2}\\ -\frac{\left(0.2209\, \sin \left(\mathrm{x5}\right)\, {\mathrm{x6}}^2 + 15.8538\, \mathrm{u1} - 44.1705\, \mathrm{x2} + 4.6107\, \cos\!\left(\mathrm{x5}\right)\, \sin\!\left(\mathrm{x5}\right)\right)}{0.47\, {\cos\!\left(\mathrm{x5}\right)}^2 - 3.84}\\ \mathrm{x4}\\ -\frac{1.0\, \left(0.2209\, \sin\!\left(\mathrm{x7}\right)\, {\mathrm{x8}}^2 + 15.8538\, \mathrm{u2} - 43.0223\, \mathrm{x4} + 4.6107\, \cos\!\left(\mathrm{x7}\right)\, \sin\!\left(\mathrm{x7}\right)\right)}{0.47\, {\cos\!\left(\mathrm{x7}\right)}^2 - 2.13}\\ \mathrm{x6}\\ \frac{0.2209\, \cos\!\left(\mathrm{x5}\right)\, \sin\!\left(\mathrm{x5}\right)\, {\mathrm{x6}}^2 + 37.67\, \sin\!\left(\mathrm{x5}\right) + 15.8538\, \mathrm{u1}\, \cos\!\left(\mathrm{x5}\right) - 44.1705\, \mathrm{x2}\, \cos\!\left(\mathrm{x5}\right)}{0.2209\, {\cos\!\left(\mathrm{x5}\right)}^2 - 1.8048}\\ \mathrm{x8}\\ \frac{0.2209\, \cos\!\left(\mathrm{x7}\right)\, \sin\!\left(\mathrm{x7}\right)\, {\mathrm{x8}}^2 + 20.8953\, \sin\!\left(\mathrm{x7}\right) + 15.8538\, \mathrm{u2}\, \cos\!\left(\mathrm{x7}\right) - 43.02\, \mathrm{x4}\, \cos\!\left(\mathrm{x7}\right)}{0.2209\, {\cos\!\left(\mathrm{x7}\right)}^2 - 1.0011} \end{array}\right)
%\end{equation}
